# Supplementary material for: The Two Faces of Capacitance: New Interpretations for Electrical Impedance Measurements of Perovskite Solar Cells and Their Relation to Hysteresis
Source: arXiv:1807.00954 ancillary file (2018-12-04)
Supplement: Supplementary file 1 [file Suppinfo_revtex.pdf]

# **The Two Faces of Capacitance: New Interpretations for Electrical Impedance Measurements of Perovskite Solar Cells and Their Relation to Hysteresis**

## **Supporting Information**

Daniel A. Jacobs,\* Heping Shen, Florian Pfeffer, Jung Peng, Thomas P. White, Fiona J. Beck, and Kylie R. Catchpole  
*Research School of Engineering, The Australian National University, Canberra, ACT 2601, Australia.*

(Dated: November 14, 2018)

## EXPERIMENTAL DETAIL

The cells fabricated for this study included those based on MAPbI<sub>3</sub> and multi-cation perovskites (Cs<sub>0.07</sub> Rb<sub>0.03</sub> FA<sub>0.765</sub> MA<sub>0.135</sub> Pb I<sub>2.55</sub>Br<sub>0.45</sub>), and were fabricated according to previously reported processes that generally result in high performing devices [1, 2]. The compact TiO<sub>2</sub> layer, of primary relevance to the C-V study of the main text, was made by spin-coating the TiO<sub>2</sub> precursor containing a titanium isopropoxide (TTIP) IPA solution and a diluted HCl IPA solution at a speed of 5000 rpm. The film thickness was controlled by varying the spin-coating times, and followed by annealing at 115° C. Each spinning cycle resulted in a TiO<sub>2</sub> film with thickness of 30±5 nm, and was repeated for the experiment reported in Figure S1c to obtain the thicker compact layers. After completing all spin-coating cycles, the film was subsequently annealed at 500° with a high oxygen pressure for 5 mins and in air for another 25 mins. For the mesoporous structure, a 70-80 nm-thick mesoporous titania layer was deposited on top of the cp-TiO<sub>2</sub> film by spin-coating diluted TiO<sub>2</sub> paste (30 NR-D) solution in ethanol (weight ratio of 1:12) at 5000 rpm for 25 s with an acceleration rate of 5000 rpm/s. The films were then sintered at 500° for 30 min in air and then left to cool.

EIS measurements were conducted on a Keysight B1500A Semiconductor Parameter Analyzer using the WGFMU unit and in-house software. High-frequency C-V measurements were conducted using the unit's dedicated capacitance meter.

## MODEL DESCRIPTION

The full set of parameters used in the main text figures is given in table S1. At the mathematical level the IDD theory addressed in this paper comprises the standard semiconductor equations coupled to a specified number of drift-diffusing ionic species, which are assumed to act simply as a mobile charge density (i.e. do not act as recombination centres, trap charge or interact chemically). It is therefore largely the same as the models employed recently by several groups to explain the phenomenology of I-V hysteresis [3–6]. One important difference is our choice to specifically include the selective contact layers in the drift-diffusion calculations. Without further modifications this drastically impacts the capacitance associated with ionic accumulation (the ion-electrode capacitance discussed in the main text) relative to a metallic boundary condition, as was used or suggested previously [4, 7, 8]. To obtain ion-electrode capacitances that are at least comparable to the ones derived from experiment, surface states were added to each absorber/contact layer interface in some of the simulations. The occupancy of these states (donors at the ETL interface and acceptors on the HTL side) was presumed to follow the instantaneous quasi-fermi level of the majority carrier on the contact side. A constant density of states per unit energy was assumed, which is denoted by the symbol  $D_{it}$  in table S1 and in Figs. 2, 3 of the main text.

Simulations of EIS/capacitance measurements were carried out by computing equilibrium solutions at the specified voltage and illumination level (relaxed for several thousand seconds), before calculating the time-domain response to a sinusoidal voltage perturbation. The implementation was made using COMSOL Multiphysics® with MATLAB LiveLink™. Fourier transformation of the time-domain data was then used to calculate all frequency-domain quantities related to the admittance.

We note that the neglect of any ionic generation-recombination mechanisms in our models, although the norm established by prior studies, is an approximation made for the sake of simplicity. Local variations in the ion concentration due to the applied voltage perturbations in EIS should, on a long enough timescale, be balanced by creation-annihilation reactions at interfaces or in the bulk. Under the hypothesis of MAI Schottky disorder the neglect of these reactions is equivalent to assuming a slow exchange of MAI with the adjacent contact layers, since the creation or destruction of an MA<sup>+</sup>/I<sup>-</sup> vacancy pair requires exchange of MAI with the environment. If instead Frenkel-type disorder were assumed dominant, a more appropriate approach might be to impose equilibrium between the formation and destruction of vacancy/interstitial defect pairs locally, as is typically assumed in modelling mixed ionic electronic conductors [11]. We do not consider such extensions of the usual IDD model here.

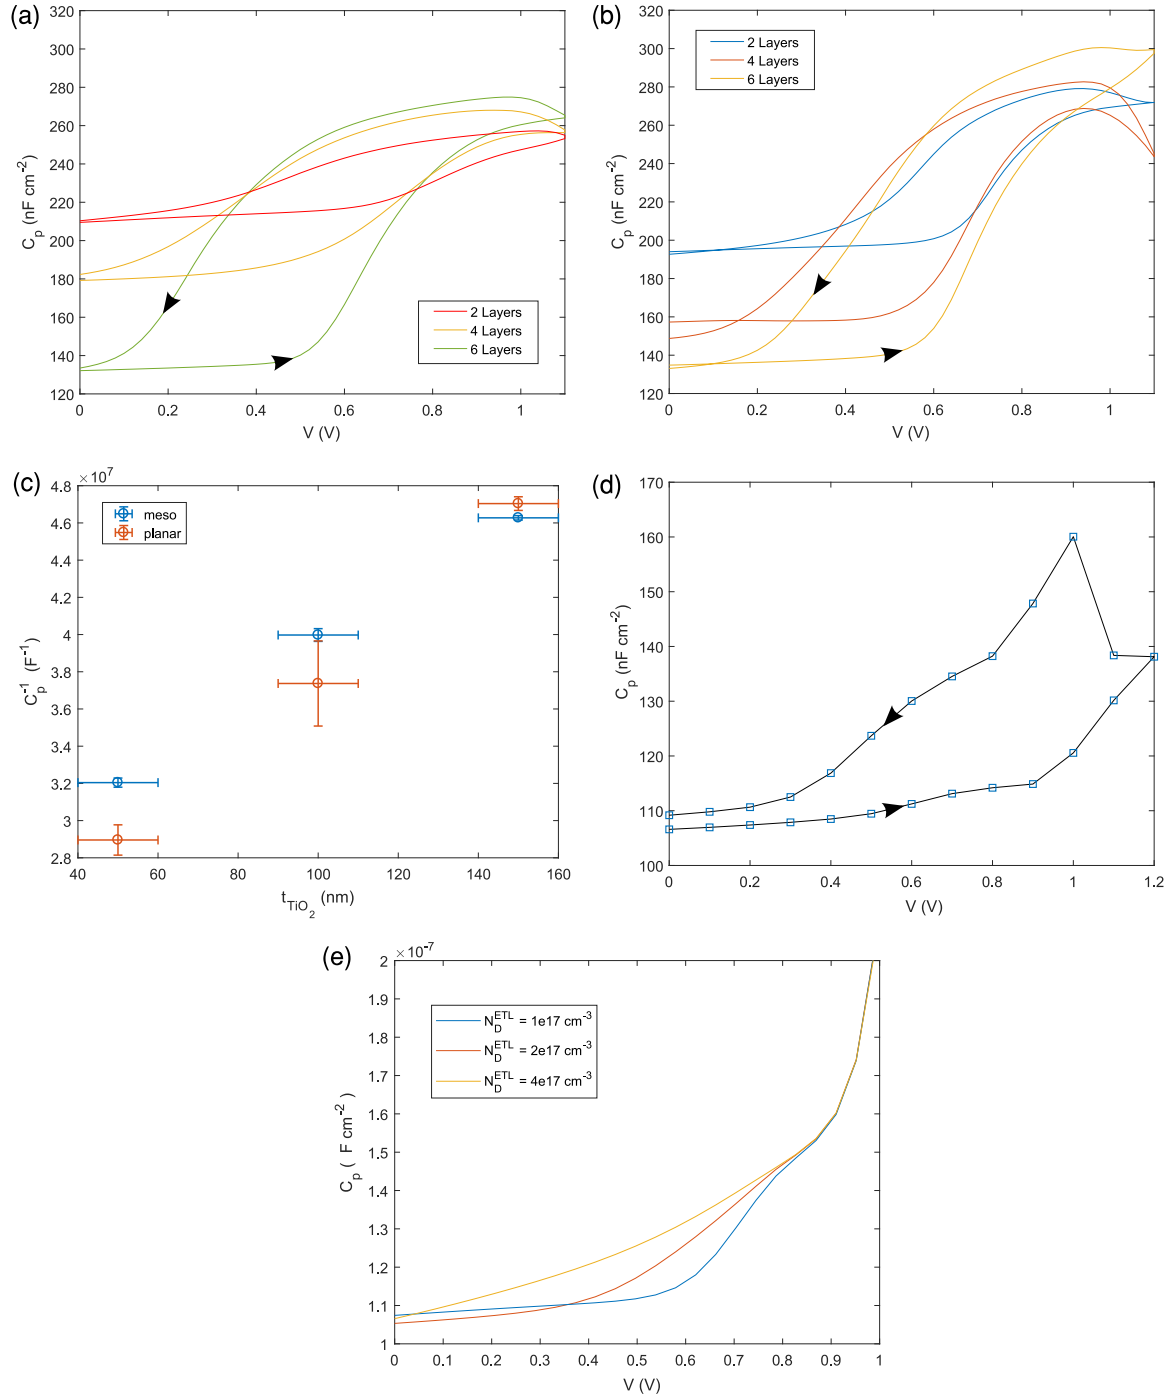

FIG. S1. (a,b) C-V measurements at 10kHz of FTO/TiO<sub>2</sub>/MAPbI<sub>3</sub>/Spiro-OMeTAD/Au cells with varying compact layer thickness. Shown for (a) no mesoporous layer (planar cells) and (b) a  $\approx 70$  nm mesoporous layer, with one representative for each condition (a minimum of 2 devices for each were tested). Measurements were performed under dark conditions using a scan-rate of  $\approx 20 \text{ mV s}^{-1}$  (i.e. faster than the rate of  $0.7 \text{ mV s}^{-1}$  used in the measurements of Fig. 4a). The measurements of (a-c) were made on a separate batch of cells to the one given in the main text of Fig. 4, and apparently feature smaller absorber thicknesses as manifested by the larger capacitance values. (c) Average capacitance at 0V for all cells versus the compact layer thickness, estimated in the abscissa to within  $\pm 10$  nm. (d) Simulated C-V at 10kHz using the model of Fig. 4b in the main text, this time with a significant scan-rate. These models qualitatively reproduce the hysteresis behaviour seen in measurements. (e) Simulations as in Fig. 4b with varying doping levels in the ETL (TiO<sub>2</sub>) layer.

| Parameter                                     | Layer      | Value(s)                                                                                                | Figures    | Description                 |
|-----------------------------------------------|------------|---------------------------------------------------------------------------------------------------------|------------|-----------------------------|
| $N_A - N_D$ (cm <sup>-3</sup> )               | ABS        | 0, $4 \times 10^{17}$ , 0                                                                               | 1, 3, 4-5  | Net doping                  |
| $\epsilon_r$                                  | ABS        | 62 [12]                                                                                                 | All        | Permittivity                |
| $E_g$ (eV)                                    | ABS        | 1.6                                                                                                     | All        | Band gap                    |
| $\chi$ (eV)                                   | ABS        | 3.9                                                                                                     | All        | Electron affinity           |
| $N_c, N_v$ (cm <sup>-3</sup> )                | ABS        | $8 \times 10^{18}$ , $6 \times 10^{18}$                                                                 | All        | Density of states           |
| $t$ (nm)                                      | ABS        | 300, 500, 500, 350                                                                                      | 1, 3, 4, 5 | Mobility                    |
| $\mu_n$ (cm <sup>2</sup> V <sup>-1</sup> s)   | ABS        | 1                                                                                                       | All        | Mobility                    |
| $\mu_p$ (cm <sup>2</sup> V <sup>-1</sup> s)   | ABS        | 1                                                                                                       | All        | Mobility                    |
| $\sigma_n$ (cm <sup>-2</sup> )                | ABS        | $1 \times 10^{-15}$                                                                                     | All        | SRH Cross-section           |
| $\sigma_p$ (cm <sup>-2</sup> )                | ABS        | $1 \times 10^{-17}$                                                                                     | All        | SRH Cross-section           |
| $N_{td}$ (cm <sup>-3</sup> )                  | ABS        | $1 \times 10^{14}$ , $1 \times 10^{14}$ , $1 \times 10^{14}$ to $1 \times 10^{16}$ , $1 \times 10^{15}$ | 1, 3, 4, 5 | Defect Density (Donor type) |
| $E_t$                                         | ABS        | mid-gap                                                                                                 | All        | SRH Energy                  |
| $N_{ion}$ (cm <sup>-3</sup> )                 | ABS        | $1 \times 10^{19}$ , $2 \times 10^{18}$ , $1 \times 10^{18}$ , $1 \times 10^{19}$                       | 1, 3, 4, 5 | SRH Energy                  |
| $D_1$ (cm <sup>2</sup> s <sup>-1</sup> )      | ABS        | $1 \times 10^{-10}$ , $1 \times 10^{-9}$ , to $1 \times 10^{-11}$ , $1 \times 10^{-11}$                 | 1, 3, 4, 5 | Ionic Diff. Const. (fast)   |
| $D_2$ (cm <sup>2</sup> s <sup>-1</sup> )      | ABS        | $1 \times 10^{-13}$ , 0, 0, 0                                                                           | 1, 3, 4, 5 | Ionic Diff. Const. (slow)   |
| $N_D$ (cm <sup>-3</sup> )                     | ETL        | $1 \times 10^{17}$ , $1 \times 10^{17}$ to $6 \times 10^{18}$ , $1 \times 10^{17}$                      | 1-2, 4, 5  | Net doping                  |
| $\epsilon_r$                                  | ETL        | 55, [13] 24 [14]                                                                                        | 1-4, 5     | Permittivity                |
| $E_g$ (eV)                                    | ETL        | 3.39                                                                                                    | All        | Band gap                    |
| $\chi$ (eV)                                   | ETL        | 4.1                                                                                                     | All        | Electron affinity           |
| $N_c, N_v$ (cm <sup>-3</sup> )                | ETL        | $8 \times 10^{18}$ , $6 \times 10^{18}$                                                                 | All        | Density of states           |
| $t$ (nm)                                      | ETL        | 120                                                                                                     | All        | Thickness                   |
| $\mu_n$ (cm <sup>2</sup> V <sup>-1</sup> s)   | ETL        | 0.1                                                                                                     | All        | Mobility                    |
| $\mu_p$ (cm <sup>2</sup> V <sup>-1</sup> s)   | ETL        | 0.1                                                                                                     | All        | Mobility                    |
| $N_A$ (cm <sup>-3</sup> )                     | HTL        | $1 \times 10^{19}$                                                                                      | All        | Net doping                  |
| $\epsilon_r$                                  | HTL        | 3                                                                                                       | All        | Permittivity                |
| $E_g$ (eV)                                    | HTL        | 3.0                                                                                                     | All        | Band gap                    |
| $\chi$ (eV)                                   | HTL        | 2.1                                                                                                     | All        | Electron affinity           |
| $N_c, N_v$ (cm <sup>-3</sup> )                | HTL        | $8 \times 10^{18}$ , $6 \times 10^{18}$                                                                 | All        | Density of states           |
| $t$ (nm)                                      | HTL        | 200                                                                                                     | All        | Thickness                   |
| $\mu_n$ (cm <sup>2</sup> V <sup>-1</sup> s)   | HTL        | 0.1                                                                                                     | All        | Mobility                    |
| $\mu_p$ (cm <sup>2</sup> V <sup>-1</sup> s)   | HTL        | 0.1                                                                                                     | All        | Mobility                    |
| $v_n$ (cm s <sup>-1</sup> )                   | ABS-ETL    | $1 \times 10^4$ , 10, $1 \times 10^{-3}$ to $1 \times 10^2$ , $1 \times 10^4$                           | 1, 2, 3, 5 | Recombination velocity      |
| $v_p$ (cm s <sup>-1</sup> )                   | ABS-ETL    | $1 \times 10^4$ , 10, $1 \times 10^{-3}$ to $1 \times 10^2$ , $1 \times 10^4$                           | 1, 2, 3, 5 | Recombination velocity      |
| $E_t$                                         | ABS-ETL    | mid-gap                                                                                                 | All        | SRH energy                  |
| $D_{it}$ (cm <sup>-2</sup> eV <sup>-1</sup> ) | ABS-ETL    | $3 \times 10^{14}$ , 0 to $3 \times 10^{14}$ , 0                                                        | 1, 2, 3-5  | Trap density                |
| $v_n$ (cm s <sup>-1</sup> )                   | HTL-ABS    | $1 \times 10^4$ , 10, $1 \times 10^{-3}$ to 1, $1 \times 10^4$                                          | 1, 2, 3, 5 | Recombination velocity      |
| $v_p$ (cm s <sup>-1</sup> )                   | HTL-ABS    | $1 \times 10^4$ , 10, $1 \times 10^{-3}$ to 1, $1 \times 10^4$                                          | 1, 2, 3, 5 | Recombination velocity      |
| $E_t$                                         | HTL-ABS    | mid-gap                                                                                                 | All        | SRH energy                  |
| $D_{it}$ (cm <sup>-2</sup> eV <sup>-1</sup> ) | HTL-ABS    | $3 \times 10^{14}$ , 0                                                                                  | 1, 2-5     | Trap density                |
| $\phi_m$ (eV)                                 | metal(ETL) | 4.4                                                                                                     | All        | Work function               |
| $\phi_m$ (eV)                                 | metal(HTL) | 5                                                                                                       | All        | Work function               |

TABLE S1. Device parameters used in our EIS simulations, chosen to emulate a “normal-structure” TiO<sub>2</sub>/MAPbI<sub>3</sub>/Spiro-OMeTAD cell. Values without references are estimates, with ranges chosen for illustrative purposes.

### Ionic Compensation of Dopants

In the main-text discussion of loop features (Figure 3) it was stated that a doping density comparable to the mean ion concentration was necessary to induce a significant bulk carrier density. In Fig. S2 this is justified by showing calculations of the bulk carrier density using our models under varying doping concentration, for a fixed (high) ion density. It can be seen that the majority carrier density falls significantly below the doping density whenever the doping is small compared to the ion density. Therefore, in simulating the loop feature we chose slightly lower ion densities ( $N_A = 4 \times 10^{17} \text{ cm}^{-3}$  with  $N_{ion} = 1 \times 10^{18} \text{ cm}^{-3}$ ) so that a significant carrier concentration could be obtained without a drastically large doping concentration.

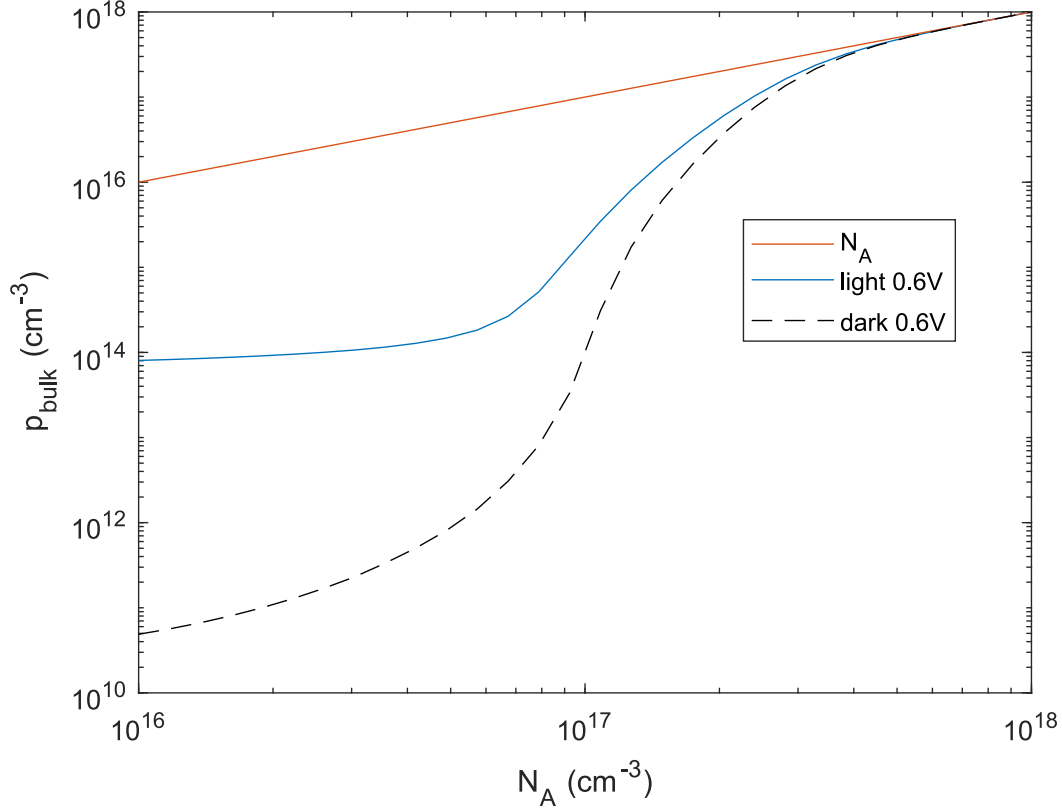

FIG. S2. Simulated majority carrier density at a mid-point in the absorber layer, versus the homogeneous density of bulk acceptors under illumination (blue solid) and darkness (black dashed). The carrier density is seen to fall significantly below the density of dopants for doping concentrations much less than the ion density (here  $1 \times 10^{19} \text{ cm}^{-3}$ ). Spatial variation of carrier densities in the bulk is minimal due to the screening effect of mobile ions.

### Ion-Electrode Capacitance

As discussed in the main text (see also Figure S3), the un-illuminated low-frequency capacitance of normal-structure cells reaches values of  $1 - 10 \mu\text{F cm}^{-2}$  at zero bias between  $10 - 100 \text{ mHz}$ . Time-domain discharge measurements on the same cell type over 1000s charge-discharge cycles (effectively probing the  $1 \text{ mHz}$  range) yield integral capacitances as large as  $80 \mu\text{F cm}^{-2}$  (such discharge measurements are a more direct way of accessing the fundamental ion-electrode capacitance since there is no contribution from recombination currents when the discharge is measured at  $0 \text{ V}$ ) [15]. In the IDD theory this capacitance is supposed to result from the accumulation of bulk ions in diffuse layers near the (ionically blocking) selective contact layers, as in the simplified Guoy-Chapmann theory of metal-electrolyte

interfaces [4]. However, one of the many differences between metal-electrolyte interfaces and those in a perovskite cell is that the carrier-selective contacts in the latter are doped semiconductors rather than metals. Ions accumulated in the diffuse layers should therefore be compensated on the contact side by either an excess of majority carriers, or else by depletion-layer space charges, which will incur their own series contribution to the total capacitance. Since depletion capacitance are typically less than  $1 \mu\text{F cm}^{-2}$ , the large low-frequency capacitance is not compatible with ionic compensation by depletion-layer space charges unless the contact layers are doped at unrealistically high levels. To the contrary, as discussed in the final section on C-V measurements there is considerable evidence that the titania layer in our normal-structure cells is almost entirely depleted at 0V, owing to modest doping densities coupled with the effect of ion accumulation. Since free electrons in the titania layer are primarily located beyond the edge of the depletion zone, some tens to hundreds of nanometers away from the interface, a large capacitance can only result if the charges compensating accumulated ions at the interface are not free carriers (i.e. they must be trapped). This is far from a surprising conclusion as anatase  $\text{TiO}_2$  is famous for having a high density of reactive surface sites [16], and surface treatments have a clear effect on the low frequency capacitance as seen in measurements of passivated cells (Figure S3). Based on the available evidence, the implicated surface states (or traps) could be intrinsic to the titania surface, the perovskite surface, hybridized orbitals, or bound states located on the ions themselves. Observations of bonding between iodine and atoms on the titania surface also suggest that a realistic picture should include a Helmholtz layer of adsorbed ions on the titania surface [17]. The Spiro interface is equally important for the ion-electrode capacitance since it contributes in series, but we are not aware of any comparable evidence in favour of surface states there. KPFM studies do indicate partial depletion however [18], so a comparable mechanism for accommodating charge is also required. A compelling possibility is provided by observations that the Spiro layer is highly permeable to extrinsic ions, including  $\text{I}^-$ ,  $\text{Li}^+$  and  $\text{H}^+$  [17, 19, 20]. Any one of these ions, if capable of moving in both the perovskite and titania layers on the relevant timescales, would short out the depletion capacitance of the Spiro layer and so potentially explain the large ion-electrode capacitance. Instead of attempting to model ion permeation into the contact layers, the simulation of Figure 1b includes surface states at both the titania and Spiro interfaces, which allow a large ion-electrode capacitance to develop given the high ion density ( $1 \times 10^{19} \text{ cm}^{-3}$ ).

### CONTINUITY EXPRESSIONS FOR THE ADMITTANCE

The following is concerned with the derivation and generalization of expression (1) given in the main text for the AC admittance of a solar cell. The starting point is the continuity equation for electrons (in the following it is understood that analogous expressions apply for holes), which in 1D and in the time-domain takes the form

$$e \frac{\partial n}{\partial t} = \frac{d}{dx} j_n - e U_n$$

where  $U_n$  is a term encompassing all sources and sinks including photo-generation, recombination, capture and emission. Linearizing, moving to the frequency domain ( $n = n_0 + \hat{n} e^{i\omega t}$ ) and rearranging

$$\frac{d}{dx} \hat{j}_n = i\omega e \hat{n} + e \hat{U}_n. \quad (1)$$

For a device with two metallic terminals located at  $x = 0, L$ , the terminal current  $\hat{I} = Y$  will generally be expressed in terms of both carrier currents plus a displacement contribution (ionically blocking terminals are assumed), such that

$$Y = \hat{j}_n(0) + \hat{j}_p(0) + \hat{j}_d(0) = \hat{j}_n(L) + \hat{j}_p(L) + \hat{j}_d(L).$$

In a device with ideal selective contact layers it is assured that only one of the carrier currents is non-negligible beyond the selective boundary. Suppose first of all that just a single electron-selective layer exists adjoining the terminal at  $x = L$  (the  $x = 0$  terminal being in contact with the absorber layer), then integration of (1) gives:

$$\begin{aligned} Y &= \hat{j}_n(L) + \hat{j}_d(L) + \hat{j}_p(L) \xrightarrow{0} \\ &= \hat{j}_n(0) + i\omega \int e \hat{n} dx + \int e \hat{U}_n dx + \hat{j}_d(L) \end{aligned} \quad (2)$$

In this case the first term relates to both the recombination of photogenerated electrons at the p-type contact, and to injection of electrons (mostly relevant at reverse bias). Either way this term conceptually belongs with the  $U_n$  since it represents a sustainable source of current. Alternatively if there is also a hole-selective layer adjoining the  $x = 0$  terminal then  $j_n(0)$  simply vanishes. Similar arguments apply to the case where there is only a selective contact on the n-side. The displacement term on the other hand can be related to the surface charge density (equivalently electron density) on the surface of the metallic terminal  $\hat{n}_s$  via Gauss's law as

$$\hat{j}_d(L) = i\omega \epsilon \epsilon_0 \hat{E}(L) = -i\omega e \hat{n}_s \quad (3)$$

and therefore conceptually belongs with the carrier density integral where it can be included as a delta source. Jointly these two simplifications leave only two terms in the admittance decomposition, one relating to accumulated charge and the other to sources of recombination (possibly including injection at metallic contacts) as in equation (1) of the main text.

When sub-gap defects are involved, one might consider it desirable to distinguish the component of  $U_n$  relating to capture and emission of electrons, which resembles a charge storage process, from some suitably defined recombination rate. This soon runs into difficulty however, as can be seen by examining the most natural splitting of  $U_n^d$  (for a single defect level) which extracts the defect filling rate:

$$U_n^d = \frac{\partial f_n}{\partial t} N_t + \left( U_n^d - \frac{\partial f_n}{\partial t} N_t \right) \quad (4)$$

$$= \frac{\partial f_n}{\partial t} N_t + U_p^d. \quad (5)$$

where  $N_t$  is the density of defects with occupation  $f_n$ . The problem here is that although the first term has a definite interpretation in terms of the charge stored in the defect level, the hole capture rate could refer either to recombination or capture-release. Identifying  $U_p$  as the recombination rate  $R$  also breaks symmetry between carrier types. Conversely, attempting to split off a symmetric recombination rate from  $U_n$  leaves a remainder which has no physical interpretation in terms of stored charge. It is therefore unlikely that there exists a unique resolution to this conceptual issue of distinguishing recombination events from filling of the defect levels. This is mostly a problem for the rare case where a defect behaves simultaneously as a trap and a recombination centre; generally either one or the other behaviour tends to dominate making the interpretation of  $U_{n,p}^d$  as either a charge-storage or recombination term clear. For example, a shallow electron trap implies  $U_p^d \approx 0$  in which case the  $\hat{U}_n$  in equation (2) contributes to  $Y_Q$  (the component of  $Y$  relating to charge storage) as

$$Y_Q = i\omega \int e \left( \hat{n} + N_t \hat{f}_n \right) dx \quad (6)$$

On the other hand for a deep defect level steady-state conditions require  $|\hat{U}_n| = |\hat{U}_p|$ , and so the identification  $R = U_p$  becomes less problematic, although there is still potential ambiguity in the phase. These ambiguities were not significant in any of the simulations considered in the main text, but may arise in other cases.

## THE EFFECT OF OPERATING POINT ON EIS HYSTERESIS MEASUREMENTS

The variation of susceptance with applied voltage and illumination levels is indicated in the measurements of Figs. S3a and S3b respectively, which were performed on mixed cation perovskite cells with a standard structure. We find that voltage has a strong effect the hysteresis measured by EIS, as seen in Fig. S3a. Moving to larger forward bias both increases the magnitude of hysteresis and reduces the characteristic timescale. Both trends are expected: on the one hand, it is natural for cells to exhibit higher sensitivity to voltage perturbations at large forward bias, as the carrier density increases near-exponentially, and the collection efficiency consequently drops rapidly in this range. A decrease in the characteristic timescale indicates that the differential ion-electrode capacitance is an increasing function of voltage (making the  $RC$  time-constant grow and hence the characteristic frequency diminish). An increase in the differential capacitance up to the built-in voltage ( $\approx 1$  V) agrees with well-studied models of ion accumulation [4], and is also incidentally what one would expect if a depletion-type capacitance limits  $C_{IE}$  (although as discussed this does not seem physically likely). The trend with illumination in Fig. S3b is simply another manifestation of the light-induced capacitance discussed at length in connection with the photo-induced capacitance. To re-iterate

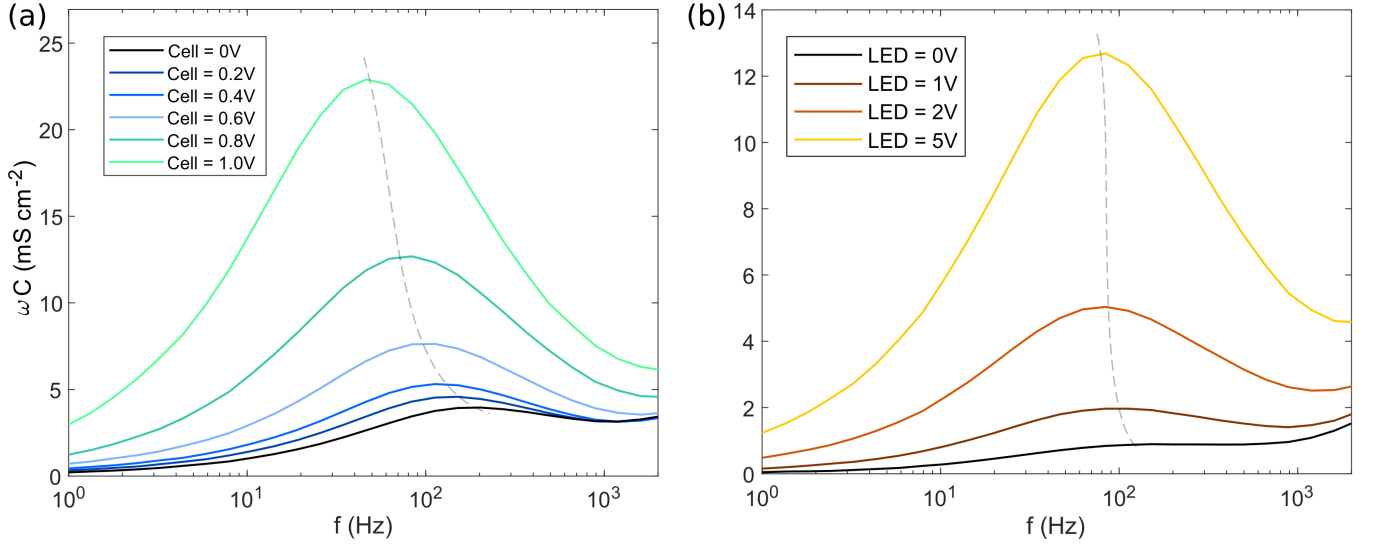

FIG. S3. Effect of applied voltage (a) and illumination intensity (b) on the susceptance of a mixed cation,  $\text{TiO}_2$ /perovskite/Spiro-OMeTAD cell. In the voltage measurement of (a) illumination was fixed at approximately 1-sun intensity (LED driver at 5 V), whereas in the illumination measurement (b) the cell was held at 0.8 V (the legend refers to the LED driver voltage, approximately linearly related to the light intensity). Dotted lines trace the evolution of the peak position (roughly the timescale of ionic relaxation) as a function of the external parameter.

the basic idea: higher carrier densities under illumination lead to an increase in recombination, whose sensitivity to voltage contributes to both the conductivity and the susceptance.

Given reports of light-enhanced ion migration in  $\text{MAPbI}_3$  [21, 22], it is interesting to note in the measurements of Fig. S3b that illumination hardly shifts the peak position (timescale) of hysteresis in mixed cation devices at all. Similar trends were observed in  $\text{MAPbI}_3$  cells. If any trend can be discerned, it is that illumination causes a decrease in the characteristic frequency, contrary to what would be expected if the illumination were acting to speed the rate of ion migration. We suggest that the conductivity measurements in refs. [21, 22] can be understood as resulting from the coupling between electronic and ionic carriers, as discussed at length in this paper, instead of changes in ionic conductivity. However, we have not explicitly considered the behaviour of lateral devices with metallic contacts here, as used in both studies, which have a much larger bulk region compared to cells, as well as differing interfaces. These will be the subject of a future investigation.

### SURFACE ROUGHNESS AND CAPACITANCE

The following concerns the interpretation of the high-frequency un-illuminated capacitance. As argued in the main-text discussion of C-V measurements (Figure 5), this quantity can be interpreted as a combination of the perovskite geometric capacitance and the contact depletion capacitance whenever the  $A_R$  contribution from injected current is negligible (i.e. at low forward bias). Between two perfectly conducting electrodes separated by a dielectric spacer of thickness  $t$  the geometric capacitance is simply  $\epsilon\epsilon_0/d$ . A question arises as to how this quantity is determined in a two-electrode system when one or more of the electrodes is non-uniform, as for example the mesoporous titania scaffold in a normal-structure perovskite cell. This is conveniently discussed in terms of the effective thickness  $t_{eff} = \epsilon\epsilon_0/C$  derived from a measurement of the capacitance assuming that the dielectric constant is known. Previously it was claimed that roughness can enhance the geometric capacitances, (equivalently reduce the effective thickness) by factors as large as 6 [23, 24]. Here we show that this is false by simulating a mesoporous electrode, and by an analytic argument showing that the effective thickness falls neatly between the capping layer thickness and the full extent of the perovskite layer. Roughness is therefore not a legitimate reason for observing abnormally large high-frequency capacitances, although it is very likely to affect the low-frequency ionic capacitance. Large high-frequency capacitance (larger than  $\approx 260 \text{ nF cm}^{-2}$ , corresponding to a small cell thickness of 200 nm with  $\epsilon \approx 60$ ) may instead be an indication of non-negligible carrier densities in the perovskite layer (i.e. net doping).

Simulations of the geometric capacitance in a 2-d geometry designed to emulate a mesoporous cell are shown in Fig S3. In the model of Fig S3 (left) the capacitance calculated in the absence of mobile ions clearly corresponds

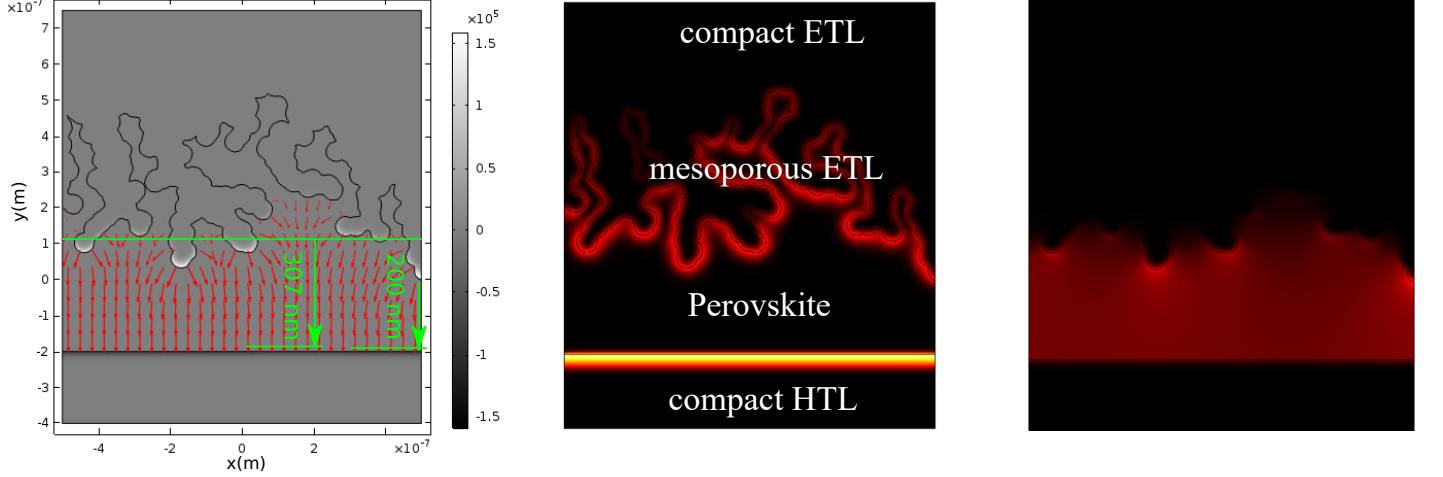

FIG. S4. (Left) Capacitance calculations in a 2-D semiconductor model with a mesoporous ETL (no mobile ions). Greyscale coloration indicates the charge density, red arrows the electric field and the green line indicates the effective geometric thickness for the calculated value of capacitance. The effective separation is found to closely approximate what would normally be regarded as the capping layer thickness. (Middle, Right) Electric field strength with and without accumulated mobile ions, respectively.

to an electric field developed over the bulk of the perovskite layer. Concentration of charge density near the tips of the mesoporous scaffold result in an effective thickness which approximates the “capping layer” thickness of the perovskite layer (Fig S3 left). Including mobile ions results in an electric field that is concentrated at the selective contact interfaces, and apparently mostly conforms to the rough mesoporous scaffold (Fig. S3 middle). Roughness can therefore be expected to enhance the ionic capacitance despite having little effect on the geometric one. Whether this effect is important for mesoporous cells will depend on the relative capacitance at the ETL and HTL interfaces, as these two contributions add in series.

A simple analytic argument confirming the insensitivity of the geometric capacitance to surface roughness is as follows. Consider a two-electrode system with one flat electrode at  $y = -d$  and another rough electrode at  $y = h(x) > 0$  with  $\min(h(x)) = 0$ . The capacitance is determined by solving the Laplace equation for the potential subject to the boundary conditions  $V(x, 0) = 0$  and  $V(x, h(x)) = \Delta V$  (the size of  $\Delta V$  is insignificant due to linearity). Equivalently it is determined via minimization of the energy equation

$$E = \frac{1}{2}C(\Delta V)^2 = \frac{1}{2\epsilon\epsilon_0} \int |\nabla V|^2 dx$$

(note that in 2D  $C$  refers to a capacitance per unit length in orthogonal direction). The minimization principle implies that any trial function  $\hat{V}$  satisfying the boundary conditions, but not necessarily the Laplace equation, obeys

$$C < \hat{C} = \frac{1}{\epsilon\epsilon_0(\Delta V)^2} \int |\nabla \hat{V}|^2 dx$$

Taking the trial function

$$\hat{V}_1 = \begin{cases} \Delta V \left( \frac{y+d}{d} \right) & y < 0 \\ \Delta V & y \geq 0 \end{cases}$$

gives

$$C < \frac{1}{\epsilon\epsilon_0 d}$$

i.e. the true capacitance is bounded by the parallel-plate capacitance with separation equal to the minimum distance between the two electrodes  $d$ . This argument assumes perfectly conducting electrodes; the true capacitance in a cell with semiconducting selective contacts will generally be lower due to the additional depletion widths.

---

\* daniel.jacobs@anu.edu.au

- [1] H. Shen, Y. Wu, J. Peng, T. Duong, X. Fu, C. Barugkin, T. P. White, K. Weber, and K. R. Catchpole, *ACS Appl. Mater. Interfaces* **9**, 5974 (2017).
- [2] J. Peng, Y. Wu, W. Ye, D. A. Jacobs, H. Shen, X. Fu, Y. Wan, N. Wu, C. Barugkin, H. T. Nguyen, *et al.*, *Energy Environ. Sci.* **10**, 1792 (2017).
- [3] S. van Reenen, M. Kemerink, and H. J. Snaith, *J. Phys. Chem. Lett.* **6**, 3808 (2015).
- [4] G. Richardson, O. S. EJ, R. G. Niemann, T. A. Peltola, J. M. Foster, P. J. Cameron, and A. B. Walker, *Energy Environ. Sci.* **9**, 1476 (2016).
- [5] P. Calado, A. M. Telford, D. Bryant, X. Li, J. Nelson, O. B. C, and P. Barnes, *Nat. Commun.* **7**, 13831 (2016).
- [6] H. Shen, D. A. Jacobs, Y. Wu, T. Duong, J. Peng, X. Wen, X. Fu, S. K. Karuturi, T. P. White, K. Weber, and K. R. Catchpole, *J. Phys. Chem. Lett.* **8**, 2672 (2017).
- [7] O. Almora, I. Zarazua, E. Mas-Marza, I. Mora-Sero, J. Bisquert, and G. Garcia-Belmonte, **6**, 1645 (2015).
- [8] N. K. Elumalai, A. Mahmud, D. Wang, M. Wright, M. B. Upama, K. H. Chan, C. Xu, and A. Uddin, *IEEE Photovoltaic Spec. Conf.*, 43rd (2016), 10.1109/PVSC.2016.7749706.
- [9] A. Walsh, D. Scanlon, S. Chen, and X. Gong, *Angew. Chem., Int. Ed.* **54**, 1791 (2015).
- [10] C. Eames, J. M. Frost, P. R. Barnes, O. B. C, A. Walsh, and S. M. Islam, *Nat. Commun.* **6**, 7497 (2015).
- [11] J. Maier, *Physical chemistry of ionic materials: ions and electrons in solids* (John Wiley & Sons, 2004).
- [12] I. Anusca, S. Balčiūnas, P. Gemeiner, Š. Svirskas, M. Sanlialp, G. Lackner, C. Fettkenhauer, J. Belovickis, V. Samulionis, M. Ivanov, *et al.*, *Advanced Energy Materials* **7**, 1700600 (2017).
- [13] R. Van de Krol, A. Goossens, and J. Schoonman, *J. Electrochem. Soc.* **144**, 1723 (1997).
- [14] M. D. Stamate, *Appl. Surf. Sci.* **218**, 318 (2003).
- [15] H. Liu, C. Liang, H. Zhang, M. Sun, J. Liang, X. Zhang, C. Ji, Z. Guo, Y. Xu, and Z. He, *Jpn. J. Appl. Phys.* **56**, 090305 (2017).
- [16] U. Diebold, *Surf. Sci. Rep.* **48**, 53 (2003).
- [17] J. Carrillo, A. Guerrero, S. Rahimnejad, O. Almora, I. Zarazua, M. Elena, J. Bisquert, and G. Germà, *Adv. Energy Mater.* **6**, 1502246 (2016).
- [18] V. W. Bergmann, Y. Guo, H. Tanaka, I. M. Hermes, D. Li, A. Klasen, S. A. Bretschneider, E. Nakamura, R. Berger, and S. A. Weber, *ACS Appl. Mater. Interfaces* **8**, 19402 (2016).
- [19] R. Ginting, M. Jeon, K. Lee, W. Jin, T. Kim, and J. Kang, *J. Mater. Chem.* **5**, 4527 (2017).
- [20] Z. Li, C. Xiao, Y. Yang, S. P. Harvey, D. Kim, J. A. Christians, M. Yang, P. Schulz, S. U. Nanayakkara, C. Jiang, J. M. Luther, J. J. Berry, M. C. Beard, A. M. M, and K. Zhu, *Energy Environ. Sci.* (2017), 10.1039/C7EE00358G.
- [21] Y.-C. Zhao, W.-K. Zhou, X. Zhou, K.-H. Liu, D.-P. Yu, and Q. Zhao, *Light: Science & Applications* **6**, e16243 (2017).
- [22] G. Y. Kim, A. Senocrate, T.-Y. Yang, G. Gregori, M. Grätzel, and J. Maier, *Nature materials* **17**, 445 (2018).
- [23] A. Pockett, G. E. Eperon, T. Peltola, H. J. Snaith, A. Walker, L. M. Peter, and P. J. Cameron, *J. Phys. Chem. C* **119**, 3456 (2015).
- [24] J. Bisquert, G. Garcia-Belmonte, and I. Mora-Sero, in *Unconventional Thin Film Photovoltaics* (2016) pp. 57–106.
